# Supplementary material for: Bianisotropic metasurfaces for scattering-free manipulation of acoustic wavefronts
Source: arXiv:1711.09840 source file (2017-11-27)
Supplement: Supplementary file 1 [file Supplementary_Material.pdf]

**Supplementary material for the paper**

# "Bianisotropic metasurfaces for scattering-free manipulation of acoustic wavefronts"

Junfei Li, Chen Shen, Ana Díaz-Rubio, Sergei Tretyakov, and Steven Cummer

## Supplementary Note 1. Minimum requirements for full control of the bianisotropic response

In this supplementary section, we deeply analyze how to control the bianisotropic response with side-loaded resonators. This analysis will determine the minimum number of resonators that allows full control of the response. In the most general case, we can express any response of a reciprocal cell as

$$\begin{bmatrix} p_{\mathrm{I}} \\ p_{\mathrm{II}} \end{bmatrix} = \begin{bmatrix} Z_{11} & Z_{12} \\ Z_{12} & Z_{22} \end{bmatrix} \begin{bmatrix} \hat{n}\cdot\vec{v}_{\mathrm{I}} \\ -\hat{n}\cdot\vec{v}_{\mathrm{II}} \end{bmatrix}. \tag{S1}$$

Although bianisotropy is produced when $Z_{11} \neq Z_{22}$, full control of the response is obtained if the cell allows to control independently the three components in the impedance matrix $Z_{11}$, $Z_{12}$, and $Z_{22}$.

The basic element in our design is a side-loaded resonator. We can analyze the response of the resonator as a local impedance which produce continuity of the pressure at both sides of the resonator [ see Fig. S1(a)]. The proposed building element is a symmetric structure and consequently any bianisotropic response can be found. In order to force the asymmetric response of the cell, we can combine the effect of two different resonators separated a distance $l$. The relation between the pressure and velocity fields at both sides of the

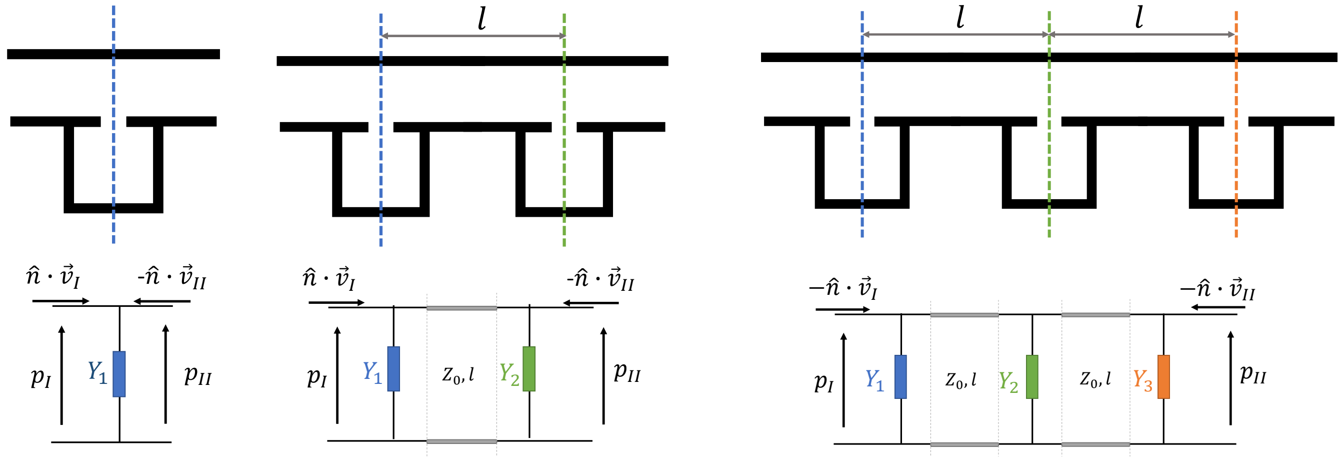


(a) (b) (c)

Figure S1: Control of the asymmetric response with side-loaded resonators. (a) Single resonators and the corresponding equivalent circuit. (b) Asymmetric cell with two resonators and the equivalent circuit. (c) Asymmetric cell with three resonators and the equivalent circuit.

cell can be written as

$$\begin{bmatrix} p_{\mathrm{I}} \\ p_{\mathrm{II}} \end{bmatrix} = \begin{bmatrix} \frac{M_{11}}{M_{21}} & \frac{1}{M_{21}} \\ \frac{1}{M_{21}} & \frac{M_{22}}{M_{21}} \end{bmatrix} \begin{bmatrix} \hat{n}\cdot\vec{v}_{\mathrm{I}} \\ -\hat{n}\cdot\vec{v}_{\mathrm{II}} \end{bmatrix}. \tag{S2}$$

where $M_{11} = \cos(kl) + jY_2\sin(kl)$, $M_{22} = \cos(kl) + jY_1\sin(kl)$, and $M_{21} = [Y_1 + Y_2]\cos(kl) + j[Y_0 + Y_2Y_1Z_0]\sin(kl)$. We can see that this structure allows bianisotropic response if $Y_1 \neq Y_2$. However, for full control of the response we need to include the separation between the resonators as a parameter of the design. This solution is not suitable for gradient metasurfaces, where the thickness of the metasurface has to be constant.

For this reason, we find that the minimum requirement for full control of the scattering properties with a constant thickness is three different resonators. If we keep the resonators equally spaced, as it is shown in

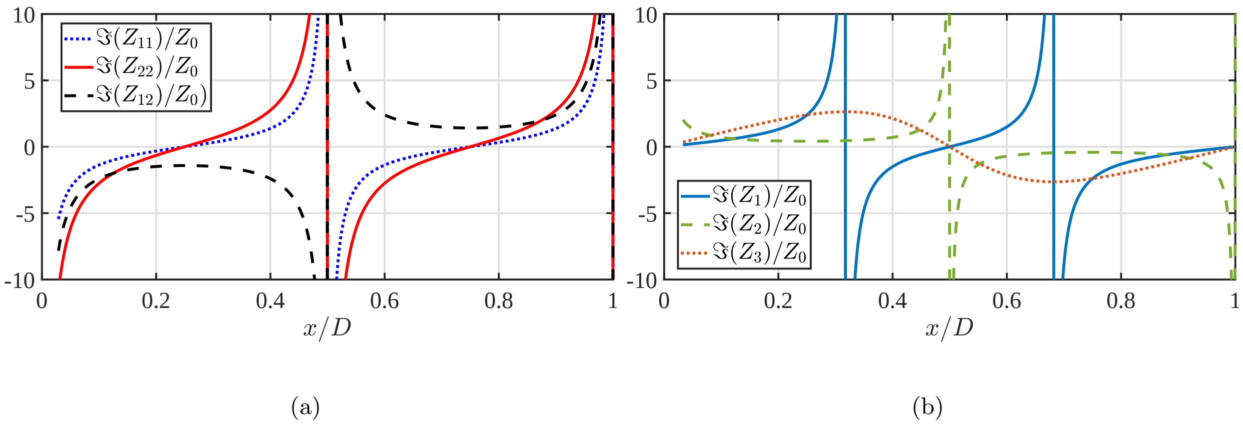


Figure S2: Gradient metasurface for anomalous refraction ($\theta_\mathrm{i} = 0°$ and $\theta_\mathrm{t} = 80°$): (a) Values of the impedance matrix in one period of the metasurface and (b) impedances of the three resonators when $l = \lambda_0/4$ which produce the desired response.

Fig. S1(c), the relation between the resonator impedances and the elements of the impedance matrix are

$$Z_1 = \frac{Z_0 \det(Z) \sin(kl)}{j \det(Z) \cos(kl) + Z_0(Z_{22} + Z_{12}) \sin(kl)} \tag{S3}$$

$$Z_2 = \frac{Z_0^2 Z_{12}(\cos(2kl) - 1)}{2 \det(Z) + 2j Z_0 Z_{12} \sin(2kl)} \tag{S4}$$

$$Z_3 = \frac{Z_0 \det(Z) \sin(kl)}{j \det(Z) \cos(kl) + Z_0(Z_{11} + Z_{12}) \sin(kl)} \tag{S5}$$

where $\det(Z) = Z_{11}Z_{22} - Z_{12}^2$. This configuration allows to independently control the three components of the impedance matrix ($Z_{11}$, $Z_{22}$, and $Z_{12}$) with a fixed thickness of the cell by changing the physical dimensions of the resonators, i.e., the values of the impedances according to Eqs. (S3-S5).

As an example, we can analyze the three-resonators model for the anomalous reflection scenario. Figure S2(a) shows the values of the impedance matrix along one period when $\theta_\mathrm{i} = 0°$ and $\theta_\mathrm{t} = 80°$. This condition can be implemented using three resonators for a fixed separation between them $l = \lambda_0/4$ if when the resonators are described by the impedances represented in Fig. S2(b). As we can see from the high impedance values at some point of the period, some of the resonators are working in the resonant frequency.

## Supplementary Note 2. Retrieving impedance matrix in COMSOL

The method we used to retrieve the impedance matrix in COMSOL is the same as the standard 4-microphone method for acoustic experiments, whose setups are shown in Fig. S2. The positions of 4 microphones are $x_1$, $x_2$, $x_3$, $x_4$, respectively. By performing two measurements with different boundary conditions at the end of the tube, we can obtain four independent equations for determination of the four transfer matrix elements. Two different boundaries we used at the end of the tube are plane wave radiation (condition #1) and hard wall (condition #2). The pressure detected by these microphones under these two boundary conditions are noted as $p_m^{(n)}$ where $m$ denotes the number of the microphone and $n$ denotes the number of the boundary condition.They satisfy the condition:

$$\begin{bmatrix} e^{-jkx_1} & e^{jkx_1} \\ e^{-jkx_2} & e^{jkx_2} \end{bmatrix} \begin{bmatrix} A^{(1)} & A^{(2)} \\ B^{(1)} & B^{(2)} \end{bmatrix} = \begin{bmatrix} p_1^{(1)} & p_1^{(2)} \\ p_2^{(1)} & p_2^{(2)} \end{bmatrix} \tag{S6}$$

Similarly,

$$\begin{bmatrix} e^{-jkx_3} & e^{jkx_3} \\ e^{-jkx_4} & e^{jkx_4} \end{bmatrix} \begin{bmatrix} C^{(1)} & C^{(2)} \\ D^{(1)} & D^{(2)} \end{bmatrix} = \begin{bmatrix} p_3^{(1)} & p_3^{(2)} \\ p_4^{(1)} & p_4^{(2)} \end{bmatrix} \tag{S7}$$

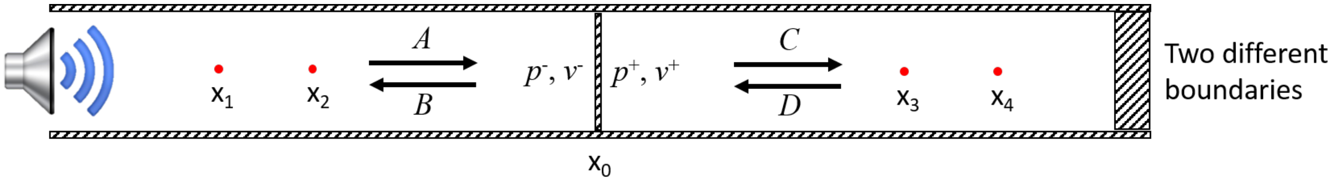


Figure S3: Setups of the standard 4-microphone method. $x_1$, $x_2$, $x_3$, $x_4$ shows the location of the microphones, $x_0$ is the location of the unit cell. $A$, $B$, $C$, $D$ shows the incoming and outgoing plane waves. Measurements are performed with two different boundaries at the end of the tube.

With the measurement of $p_m^{(n)}$, all the ABCD in the matrices can be calculated. If the metasurface is

located at $x_0$, then the pressure and velocity at the left side and right side can be written as:

$$\begin{bmatrix} p^{-(1)} & p^{-(2)} \\ v^{-(1)} & v^{-(2)} \end{bmatrix} = \begin{bmatrix} e^{-jkx_0} & e^{jkx_0} \\ e^{-jkx_0}/Z_0 & -e^{jkx_0}/Z_0 \end{bmatrix} \begin{bmatrix} A^{(1)} & A^{(2)} \\ B^{(1)} & B^{(2)} \end{bmatrix} \tag{S8}$$

$$\begin{bmatrix} p^{+(1)} & p^{+(2)} \\ v^{+(1)} & v^{+(2)} \end{bmatrix} = \begin{bmatrix} e^{-jkx_0} & e^{jkx_0} \\ e^{-jkx_0}/Z_0 & -e^{jkx_0}/Z_0 \end{bmatrix} \begin{bmatrix} C^{(1)} & C^{(2)} \\ D^{(1)} & D^{(2)} \end{bmatrix} \tag{S9}$$

Therefore, the transfer matrix of the measured unit cell can be calculated as

$$T = \begin{bmatrix} p^{+(1)} & p^{+(2)} \\ v^{+(1)} & v^{+(2)} \end{bmatrix} \begin{bmatrix} p^{-(1)} & p^{-(2)} \\ v^{-(1)} & v^{-(2)} \end{bmatrix}^{-1} \tag{S10}$$

Hence the impedance matrix can is calculated as

$$Z = \begin{bmatrix} -\frac{T_{22}}{T21} & -\frac{1}{T21} \\ \frac{T_{12}T_{21}-T_{11}T_{22}}{T21} & -\frac{T_{11}}{T21} \end{bmatrix} \tag{S11}$$

## Supplementary Note 3. Numerical simulations when loss is considered

Although the structure is designed with lossless assumption, the performance is also confirmed in simulation by considering viscous loss since it is the inherent loss of the structure which is inevitable in the experiments. Loss in the air is modeled by the viscous fluid model in the Pressure Acoustic Module in COMSOL, with dynamic viscosity of $1.82 \times 10^{-5}$Pa and bulk viscosity of $5.46 \times 10^{-2}$Pa. The simulated fields are shown in Fig. S4. The simulations show that for the bianisotropic design, the amplitude of the transmission coefficient decays to $T = 1.31$ indicating that 85% of the energy is transmitted to the desired direction. This value is still higher than lossless discretized GSL-based designs. This confirms that the performance of the designed metasurface will not be severely influenced when loss is considered. This is because the proposed metasurface is not resonant based, and all the resonators are designed so that the operating frequency is far off resonance [see Supplementary Note 6].

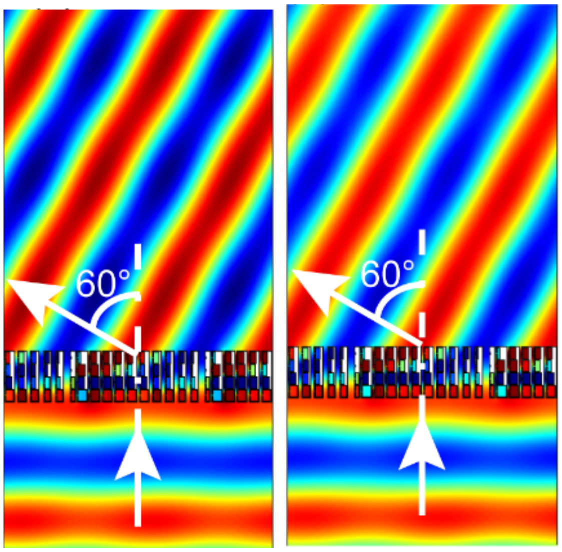


(a) (b)

Figure S4: Simulated acoustic field (real part) of the designed perfect metasurface for $\theta_\mathrm{i} = 0°$ and $\theta_\mathrm{t} = 60°$ using the proposed non-resonant structures. (a) Lossless simulation and (b) simulation with viscous loss in air.

## Supplementary Note 4. Comparison between transfer matrix method and numerical simulations

To evaluate the performance of the transfer matrix, we compare the transmission and reflection characteristics of a cell both analytically and numerically. The dimensions of the cell is the same as Fig.2 in the main text, i.e., $w = 12$ mm, $h_2 = 1.5$ mm, $w_2 = 1$ mm, $h_1 = 1$ mm $w_1 = 4$ mm, $w_\mathrm{a} = 6$ mm, $w_\mathrm{b} = 5$ mm, $w_\mathrm{c} = 4$ mm, and $w_\mathrm{d} = 3$ mm. The lines represent the results from the transfer matrix method and the markers represent numerical simulations from COMSOL. Good agreement can be observed and the results confirm the biansiotropic nature of the structure proposed, as the reflected phase from opposite directions are different.

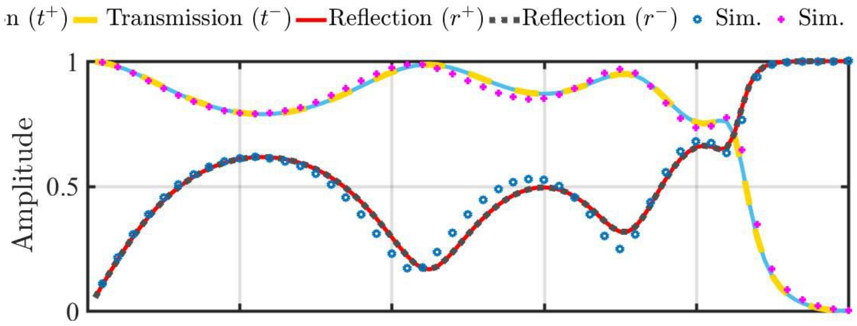


(a)

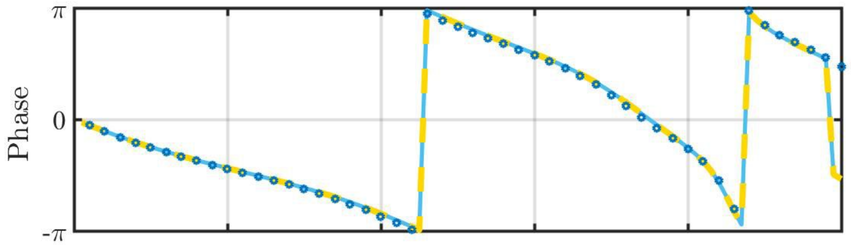


(b)

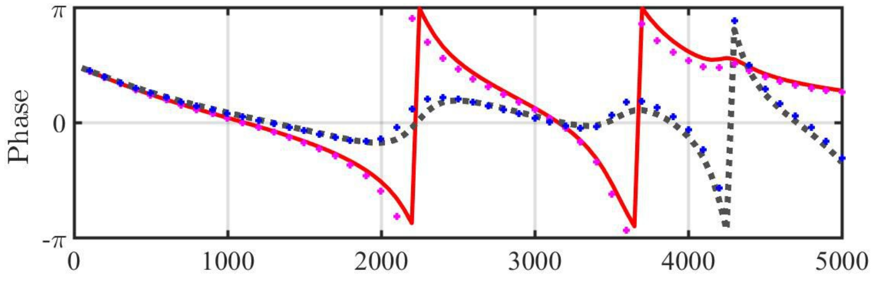


(c)

Figure S5: Comparison between transfer matrix method and numerical simulations

## Supplementary Note 5. Convergence of the optimization process in each design

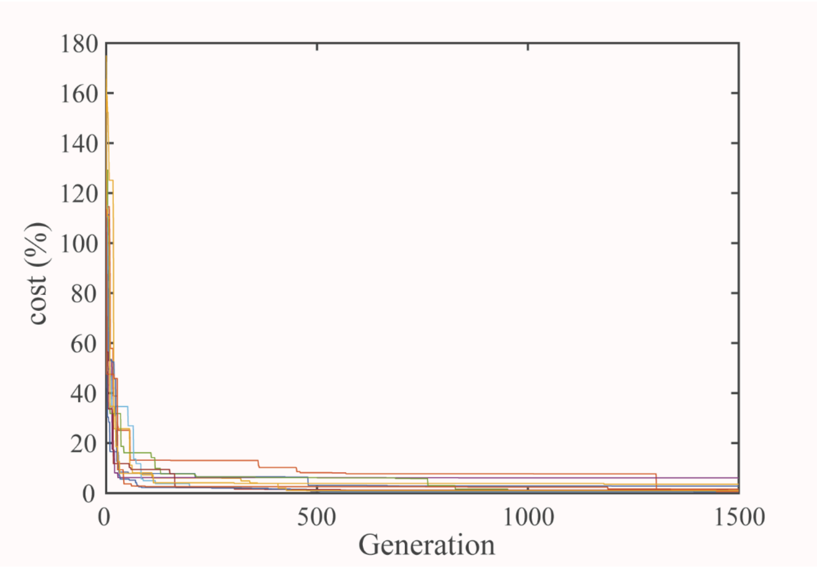


(a)

Figure S6: The evolution of the cost function with the evolution of the algorithm. The figure shows 10 convergence plots.

To show the convergence of the optimization process, the evolution of the cost function with the evolution of the algorithm for the first cell of the 60° case is shown in Supplementary Fig. 6(a) as an example. For cleanness, here we only showed 10 evolution results.

## Supplementary Note 6. Design parameters of the scattering-free anomalous refractive metasurfaces

This section details the physical dimensions of the final designs for the anomalous refractive metasurfaces when $\theta_\mathrm{i} = 0^\circ$ and $\theta_\mathrm{t} = 60^\circ$ (Table S1), $\theta_\mathrm{t} = 70^\circ$ (Table S2), and $\theta_\mathrm{t} = 80^\circ$ (Table S3).

| | | Resonator A | | Resonator B | | Resonator C | | Resonator D | |
|---|---|---|---|---|---|---|---|---|---|
| Cell | $w_1(mm)$ | $w_\mathrm{a}$ (mm) | $f_\mathrm{a}$ (kHz) | $w_\mathrm{b}$ (mm) | $f_\mathrm{b}$ (kHz) | $w_\mathrm{c}$ (mm) | $f_\mathrm{c}$ (kHz) | $w_\mathrm{d}$ (mm) | $f_\mathrm{d}$ (kHz) |
| 1 | 2.4 | 7.6 | 4.61 | 6.1 | 5.21 | 4.3 | 6.30 | 4.0 | 6.54 |
| 2 | 3.2 | 6.8 | 4.78 | 5.3 | 5.48 | 5.6 | 5.32 | 5.1 | 5.59 |
| 3 | 3.5 | 6.5 | 4.86 | 4.2 | 6.14 | 4.1 | 6.22 | 4.6 | 5.86 |
| 4 | 4.6 | 5.4 | 5.24 | 4.9 | 5.52 | 2.8 | 7.34 | 4.6 | 5.71 |
| 5 | 4.6 | 5.4 | 5.24 | 3.0 | 7.10 | 1.0 | 11.23 | 1.9 | 8.78 |
| 6 | 6.8 | 3.2 | 6.63 | 3.1 | 6.73 | 0.1 | 16.20 | 0.1 | 16.20 |
| 7 | 1.4 | 8.6 | 4.52 | 6.1 | 5.50 | 6.9 | 5.13 | 2.4 | 8.91 |
| 8 | 1.9 | 8.1 | 4.54 | 7.8 | 4.64 | 7.0 | 4.94 | 5.6 | 5.59 |
| 9 | 2.1 | 7.9 | 4.56 | 7.6 | 4.67 | 6.5 | 5.10 | 5.8 | 5.43 |
| 10 | 2.1 | 7.9 | 4.56 | 6.8 | 4.97 | 4.9 | 5.95 | 5.7 | 5.48 |
| 11 | 2.2 | 7.8 | 4.58 | 6.6 | 5.03 | 3.9 | 6.69 | 4.7 | 6.06 |

Table S1: Design parameters and resonance frequencies of the individual resonators of the scattering-free bianisotropic metasurface to steer a normal incident wave toward $\theta_\mathrm{t} = 60^\circ$, implemented with 11 cells within one period.

| Cell | cost(%) | $w$ (mm) | $w_1$ mm) | $w_a$ (mm) | $w_b$ (mm) | $w_c$ (mm) | $w_d$ (mm) |
|---|---|---|---|---|---|---|---|
| 1 | 17.42 | 30.4 | 10.4 | 9.1 | 7.5 | 11.4 | 10.2 |
| 2 | 4.50 | 30.4 | 11.9 | 6.5 | 16.2 | 8.6 | 16.0 |
| 3 | 1.52 | 30.4 | 15.6 | 9.2 | 7.2 | 2.0 | 3.5 |
| 4 | 5.94 | 30.4 | 10.9 | 10.6 | 10.6 | 5.2 | 1.7 |

Table S2: Design parameters of the individual resonators of the scattering-free bianisotropic metasurface to steer a normal incident wave toward $\theta_t = 70°$ implemented with 4 cells within one period.

| Cell | cost(%) | $w$ (mm) | $w_1$ mm) | $w_a$ (mm) | $w_b$ (mm) | $w_c$ (mm) | $w_d$ (mm) |
|---|---|---|---|---|---|---|---|
| 1 | 4.07 | 29.0 | 4.6 | 9.6 | 10.7 | 4.4 | 4.6 |
| 2 | 14.32 | 29.0 | 7.1 | 6.6 | 19.3 | 7.4 | 19.1 |
| 3 | 15.40 | 29.0 | 16.5 | 3.8 | 9.9 | 0.3 | 6.1 |
| 4 | 9.47 | 29.0 | 14.5 | 7.5 | 8.7 | 11.5 | 9.4 |

Table S3: Design parameters of the individual resonators of the scattering-free bianisotropic metasurface to steer a normal incident wave toward $\theta_t = 80°$ implemented with 4 cells within one period.
